# Supplementary material for: A boundary integral method with volume-changing objects for ultrasound-triggered margination of microbubbles
Source: arXiv:1608.05196 source file (2017-08-11)
Supplement: Supplementary file 1 [file SI.pdf]

# Supplementary information for
# "A boundary integral method with volume-changing objects for ultrasound-triggered margination of microbubbles"

Achim Guckenberger*, Stephan Gekle*

Dated: August 11, 2017

# Contents

**S1 Determination of error bars and average RBC/bubble positions** 1

**S2 Results with included radiation force** 2
S2.1 Method . . . 2
S2.2 Results for $P_A = 45\,\text{kPa}$ . . . 2
S2.3 Results for $P_A = 6\,\text{kPa}$ . . . 3

**S3 Parameter robustness** 4

**S4 Code verification** 6

**S5 Dynamic mesh refinement** 8

# S1 Determination of error bars and average RBC/bubble positions

The error bars and average positions in the figures (such as fig. 4 (b)) are determined via the following steps:

1) We take the minimum, maximum and arithmetic mean of the centroids of *all* RBCs or bubbles in the system in each time step for $t > 1\,\text{s}$ or after definite margination. This gives three graphs as a function of time, once for the set of all RBCs and once for the set of the two bubbles. See figure S1 for an illustration.

2) These time series are then averaged to obtain a mean minimal, maximal and average centroid position. See the straight horizontal lines in figure S1.

3) This is then done for all simulations with the same set of parameters. Each of the resulting six values per simulation (three for the RBCs and three for the bubbles) are then averaged over the different simulations with the considered durations as weights. This gives the final minimal, maximal and average values which are then depicted as error bars and points, respectively.

Note that this procedure is similar to the one from reference [1].

*Biofluid Simulation and Modeling, Fachbereich Physik, Universität Bayreuth, Bayreuth

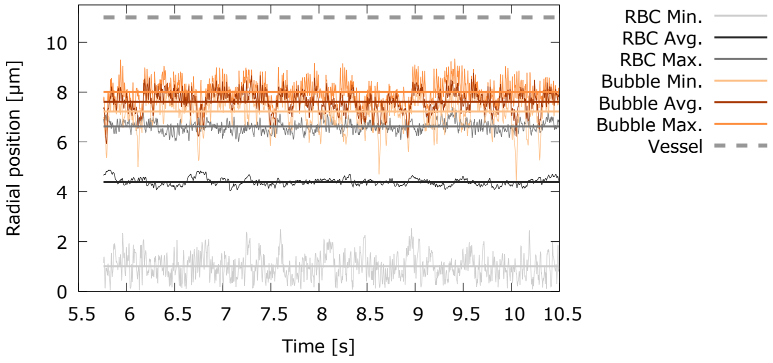


Figure S1: Illustration of the first two steps to obtain the error bars and average object positions, exemplified via the simulation from figure 4 (a) from the main text. The jagged lines show the minimal, maximal and average positions of the centroids as a function of time. The straight lines depict the corresponding temporal averages.

# S2 Results with included radiation force

As explained in the main text, bubbles under the influence of ultrasound experience so-called radiation forces [2–4]. The primary radiation force $\boldsymbol{F}_{\text{rad}}$ pushes them usually away from the sound source, while the secondary radiation force tends to attract the bubbles towards each other. They have been neglected in the main text. We include the primary radiation force here explicitly in order to show that it plays only a minor role for the parameters from the main text (which have been intentionally chosen such that *isotropic* margination dominates). The remaining system setup is identical to the standard one from section 3.2, if not noted otherwise.

## S2.1 Method

The primary radiation force is given by [5]

$$\boldsymbol{F}_{\text{rad}} = -\langle V(t) \nabla P(t) \rangle_t \,, \tag{1}$$

where $V(t)$ is the bubble volume and the pressure gradient is computed from

$$\nabla P = -\boldsymbol{k} P_{\text{A}} \cos(2\pi f t) \tag{2}$$

with the wavevector $\boldsymbol{k} = 2\pi f / c\, \hat{\boldsymbol{e}}_z$ of the incoming acoustic wave in the positive $z$-direction which is perpendicular to the vessel's axis. $f$ is the acoustic frequency and $P_{\text{A}}$ the prescribed pressure amplitude. The angular brackets indicate the temporal average. The time evolution of the bubble volume is obtained by solving the modified Rayleigh-Plesset equation given by reference [6, eq. (3)] for a single bubble numerically. Thus, the primary radiation force is computed under the assumption of negligible deformation and an infinite ambient fluid reservoir.

We solve the Rayleigh-Plesset equation in MATLAB, where we include a certain pressure amplitude $P_{\text{A}}$, a surface dilatational viscosity of $1.5 \times 10^{-8}$ kg/s, a plasma density of $\rho = 10^3\,\text{kg/m}^3$, a polytropic gas exponent of $\kappa = 1.095$ and the speed of sound $c = 1480\,\text{m/s}$ [6]. We solve it for at least 16 periods with a relative tolerance of $10^{-12}$ and an absolute tolerance of $10^{-12} R_0$ using the ode45 integrator. To prevent numerical artifacts, a small finite elastic compression modulus [6] of typically $\chi = 0.002\,\text{N/m}$ is included (we checked that the results are insensitive to the exact value of $\chi$). The remaining two parameters that need to be specified are the radii $R_0$ and $R_{\text{soft}}$. The solution then provides us with the constant force $\boldsymbol{F}_{\text{rad}}$, which is converted to a traction jump as explained by reference [7, sec. 2.3]. Otherwise, the numerical procedure is identical to the one from the main text where radiation forces are not included.

## S2.2 Results for $P_{\text{A}} = 45\,\text{kPa}$

As an example, setting $P_{\text{A}} = 45\,\text{kPa}$, $f = 1\,\text{kHz}$ and $R_0 = R_{\text{soft}} = 2\,\mu\text{m}$ as in the main text leads to $|\boldsymbol{F}_{\text{rad}}| \approx 1.2 \times 10^{-15}\,\text{N}$. Examining again the case of two bubbles without RBCs in figure S2 (a), we find that contrary to figure 8 (a) from the main manuscript some outward migration occurs. Nevertheless, the final radial position is halved compared to full margination as observed when RBCs are included (see any graphic with RBCs, e.g.

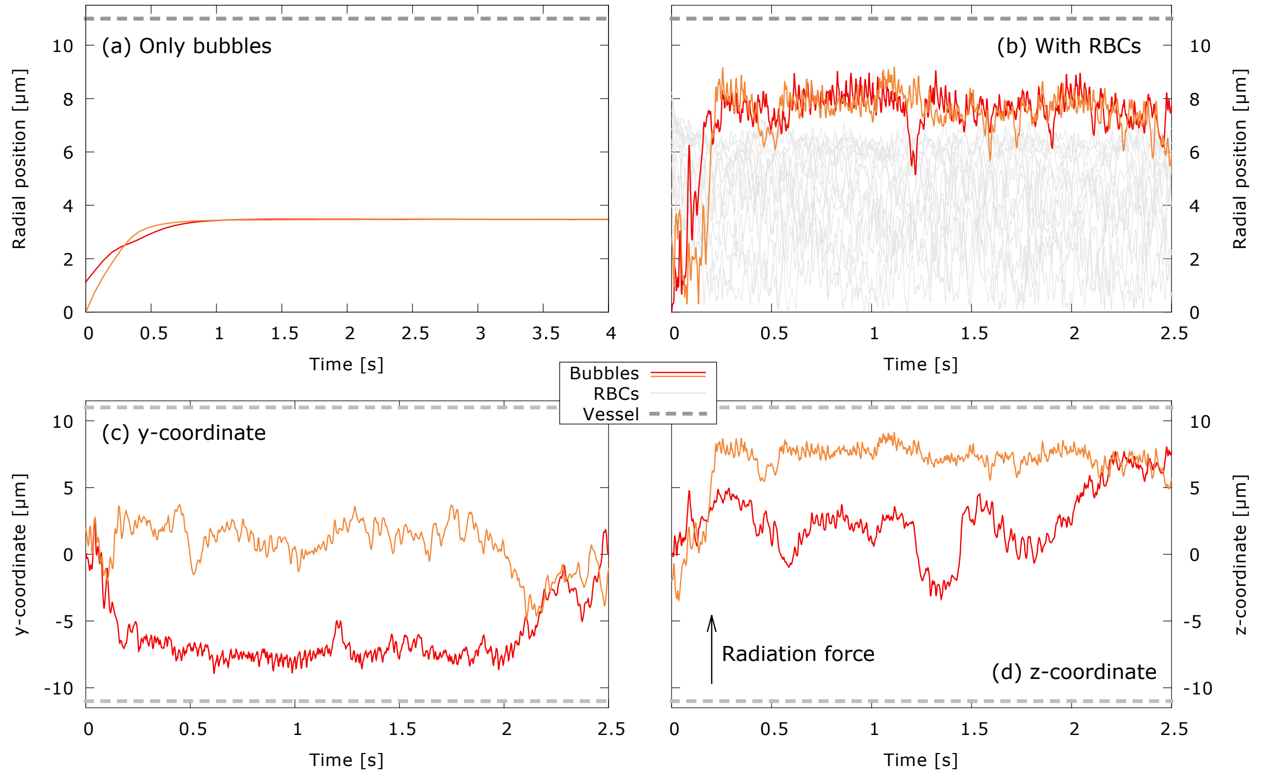


Figure S2: Radial positions of the centroids of two oscillating microbubbles ($f = 1\,\text{kHz}$, $R_{\text{eff}} \in [1.7; 2.23]\,\mu\text{m}$) that are coated with lipid molecules ($\gamma \in [0.5; 10]\kappa_S$) for $\delta = 1$. Primary radiation force for 45 kPa included in the positive $z$-direction ($|\boldsymbol{F}_{\text{rad}}| \approx 1.2 \times 10^{-15}\,\text{N}$). (a) Without red blood cells. (b) With red blood cells (hematocrit: 16 %). (c) and (d) The $y$- and $z$-coordinates of the two bubbles from (b).

figure S2 (b)). This indicates that margination due to the interactions with the RBCs is the dominating factor for the outward migration.

Including RBCs as well as the primary radiation force $\boldsymbol{F}_{\text{rad}}$ in the positive $z$-direction leads to figure S2 (b). Obviously, UTM still occurs. If this would be primarily due to the radiation force, one would expect that the bubbles are pushed in the direction of the force, i.e. in the positive $z$-direction. However, as figures S2 (c) and (d) show, the initial margination of one bubble is in the negative $y$-direction and thus perpendicular to $\boldsymbol{F}_{\text{rad}}$.

Both examples highlight that the primary radiation force plays only a secondary role for $P_A = 45\,\text{kPa}$ and $f = 1\,\text{kHz}$. For $f = 10\,\text{kHz}$, however, we find $|\boldsymbol{F}_{\text{rad}}| \approx 10^{-13}\,\text{N}$, a value which leads to a dominating influence of the radiation force. As this goes hand in hand with the undesired one-sided agglomeration away from the ultrasound source, we thus propose to reduce the pressure amplitude at higher frequencies in order to exploit the isotropy of UTM. Corresponding results will be considered next.

## S2.3 Results for $P_A = 6\,\text{kPa}$

Reducing the pressure amplitude to $P_A = 6\,\text{kPa}$, we find for $f = 1\,\text{kHz}$ and $R_0 = R_{\text{soft}} = 2\,\mu\text{m}$ a value of $|\boldsymbol{F}_{\text{rad}}| \approx 1.5 \times 10^{-17}\,\text{N}$. For the $P_A = 6\,\text{kPa}$ simulations we also extract the minimal and maximal radial excursions ($R_{\text{min}}$ and $R_{\text{max}}$, respectively) and thus the flux amplitudes $A_i$ from the solution of the Rayleigh-Plesset equation.

Without RBCs, the bubbles once again migrate to the channel center as displayed in figure S3 (a), showing that a radiation force of $|\boldsymbol{F}_{\text{rad}}| \approx 1.5 \times 10^{-17}\,\text{N}$ is indeed negligible. This is further confirmed in figure S3 (b), where RBCs are included but the effective surface tension during the oscillations is held constant: The soft bubbles remain in the center as expected. The same figure also shows (see the stiff bubbles) that the smaller pressure amplitude and thus the smaller radial excursions compared to the main manuscript do not affect the margination behavior.

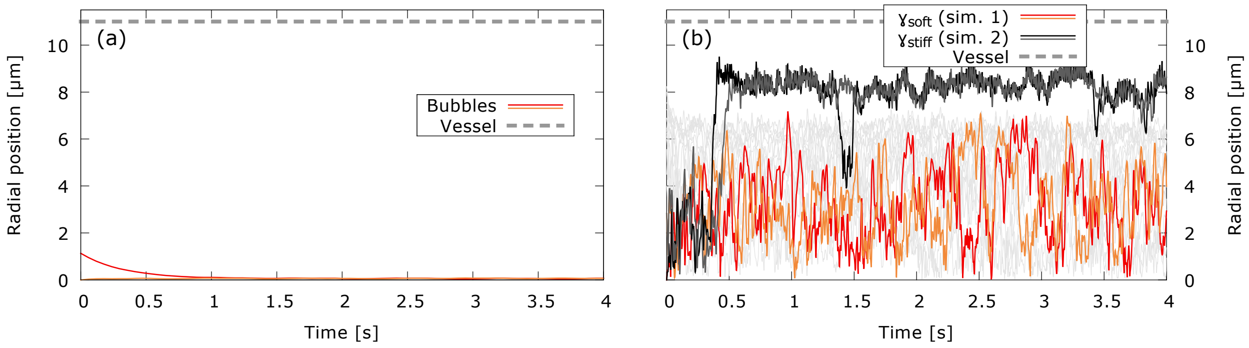


Figure S3: Radial positions of the centroids of two oscillating microbubbles ($f = 1\,\text{kHz}$, $R_{\text{eff}} \in [1.96; 2.03]\,\mu\text{m}$, $P_{\text{A}} = 6\,\text{kPa}$). Primary radiation force included ($|\boldsymbol{F}_{\text{rad}}| \approx 1.5 \times 10^{-17}\,\text{N}$). (a) Without red blood cells. Lipid-coated microbubbles, i.e. $\gamma \in [0.5; 10]\kappa_{\text{S}}$ with $\delta = 1$. (b) Margination behavior of purely soft and purely stiff oscillating microbubbles *with* RBCs. Two distinct simulations: The constant surface tensions are $\gamma = \gamma_{\text{soft}} = 0.5\kappa_{\text{S}}$ (red/orange) and $\gamma = \gamma_{\text{stiff}} = 10\kappa_{\text{S}}$ (black/gray). The hematocrit is fixed to 16%. The soft bubbles ($\gamma = \gamma_{\text{soft}}$) remain in the center, whereas the stiff bubbles ($\gamma = \gamma_{\text{stiff}}$) show margination.

We further study this case in figure S4 (a) where we show the analogous result to figure 4 (a) from the main text. After switching on the oscillations, rapid migration within less than one second is observed. The transition in figure S4 (b) roughly corresponds to figure 4 (b); some slight differences are observed as the realized trajectories are different. Moreover, figure S5 highlights that the margination is still isotropic (i.e. similar to figure 6 from the main text), despite the inclusion of the radiation force.

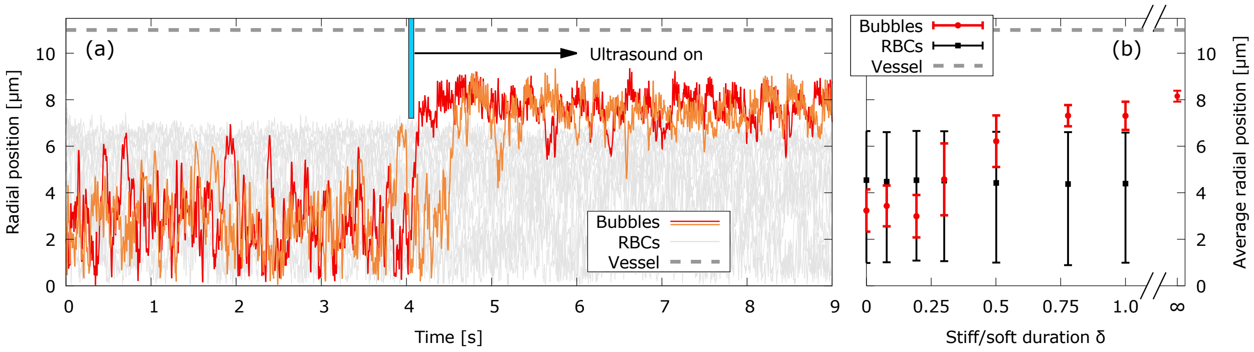


Figure S4: Ultrasound-triggered margination. Primary radiation force included for oscillating bubbles ($f = 1\,\text{kHz}$, $P_{\text{A}} = 6\,\text{kPa}$). (a) Radial positions of the centroids of two microbubbles coated with lipids. When the acoustic pressure is switched on at $\approx 4\,\text{s}$, ultrasound-triggered margination leads to rapid migration to the vessel wall. Here, $\delta = 1$, i.e. the bubbles are stiff for the first half of the ultrasound period and soft during the second one with their effective surface tension varying in the range $\gamma \in [0.5; 10]\kappa_{\text{S}}$. The effective radii alternate between $1.96\,\mu\text{m}$ and $2.03\,\mu\text{m}$. The primary radiation force is $|\boldsymbol{F}_{\text{rad}}| \approx 1.5 \times 10^{-17}\,\text{N}$. (b) Average radial positions of the oscillating bubbles and RBCs for several different values of $\delta$. Note that the rightmost point corresponds to the limit $\delta \to \infty$ (i.e. always stiff). The primary radiation force varies only slightly with $\delta$ ($|\boldsymbol{F}_{\text{rad}}| \approx 1.5 - 1.6 \times 10^{-17}\,\text{N}$). The determination of the error bars is explained in section S1.

Increasing the frequency from $f = 1\,\text{kHz}$ to $10\,\text{kHz}$ at $P_{\text{A}} = 6\,\text{kPa}$ while the primary radiation force is included leaves the qualitative results for the radial position unchanged but approximately halves the average asphericity, as depicted in figure S6. This matches with the observations from the main manuscript where no radiation forces were considered (figure 7).

# S3 Parameter robustness

Ultrasound-triggered margination is a robust effect. Figures S7 and S8 show that reducing the effective surface tension in the soft state to $\gamma_{\text{soft}} = 0.1\kappa_{\text{S}}$, increasing the stiff state tension to $\gamma_{\text{stiff}} = 25\kappa_{\text{S}}$, or changing numerical parameters such as the precision of the solver, the initial position or the length of the periodic vessel does not

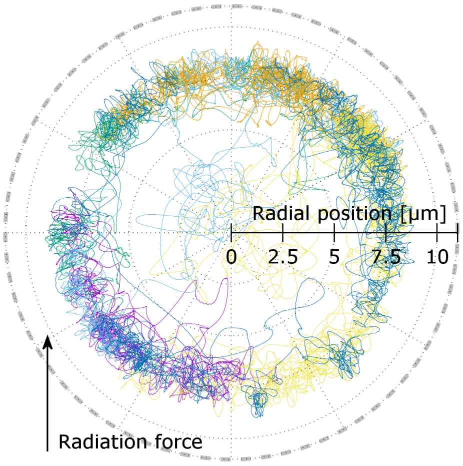


Figure S5: Polar plot of several bubble trajectories (i.e. as viewed from the outlet). The figure shows the $\delta \approx 0.78$ and $\delta = 1$ simulations used for figure S4 (b), representing different system realizations. Hence, the primary radiation force is included (for $f = 1\,\text{kHz}$ and $P_A = 6\,\text{kPa}$; direction indicated by the arrow). Trajectories only shown for $t > 1\,\text{s}$ or after definite margination. Rare short-lived migration events to the inside occur. Each bubble in each simulation is shown in a different color. The outer gray dashed line depicts the vessel radius.

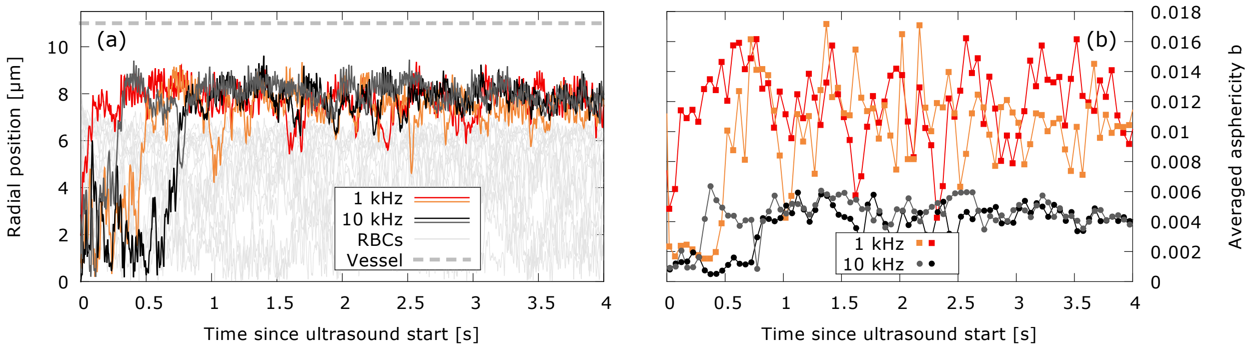


Figure S6: Behavior of two oscillating lipid coated microbubbles for $\delta = 1$ with red blood cells, once for a frequency of $f = 1\,\text{kHz}$ and once for 10 kHz (two distinct simulations; the $f = 1\,\text{kHz}$ curve is the simulation from figure S4 (a), but shown only from the beginning of the oscillations). The primary radiation force for 6 kPa is included ($|\boldsymbol{F}_{\text{rad}}| \approx 1.5 \times 10^{-17}\,\text{N}$ for 1 kHz and $|\boldsymbol{F}_{\text{rad}}| \approx 1.6 \times 10^{-15}\,\text{N}$ for 10 kHz). (a) Radial positions of the centroids. The red blood cells are shown in light gray. (b) Corresponding microbubble asphericities averaged over consecutive time intervals of 50 ms.

affect the overall results qualitatively (i.e. margination on average is still observed). Furthermore, halving the bubbles' equilibrium radius or making the vessel wall stiffer does not lead to significant changes either (fig. S8). Note that depending on the exact history, short lived migrations toward the vessel center can occur sometimes, which are nevertheless again followed by rapid movement to the vessel walls.

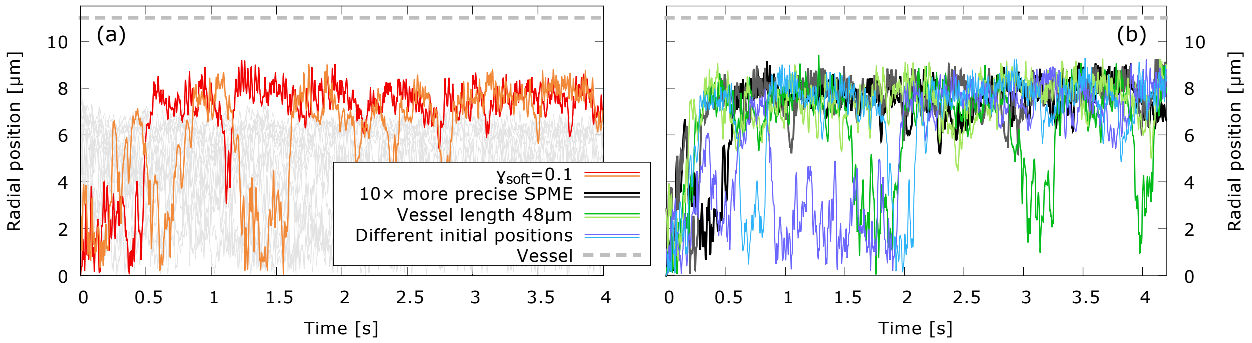


Figure S7: Radial positions of the centroids of two oscillating lipid coated microbubbles ($f = 1$ kHz, $P_A = 45$ kPa) for $\delta = 1$ with red blood cells. Radiation forces *not* included. (a) The surface tension in the soft state is reduced to $\gamma_{soft} = 0.1\kappa_S$, retaining the effect of margination without qualitative changes (red/orange). The gray lines indicate the red blood cells. (b) Three different simulations for $\gamma_{soft} = 0.5\kappa_S$: One with more precise SPME parameters (cutoff errors below $\lesssim 0.001\,\%$, i.e. one order of magnitude smaller than usual; also see section 2.5 in the main manuscript; black/gray lines), one with the larger system from figure 2 (a) from the main text (vessel length 48 µm and hematocrit 16 %; dark/light green), and one with different initial positions for all particles compared to the remaining simulations (RBCs initialized in regular arrays; purple/blue). Red blood cells omitted for clarity.

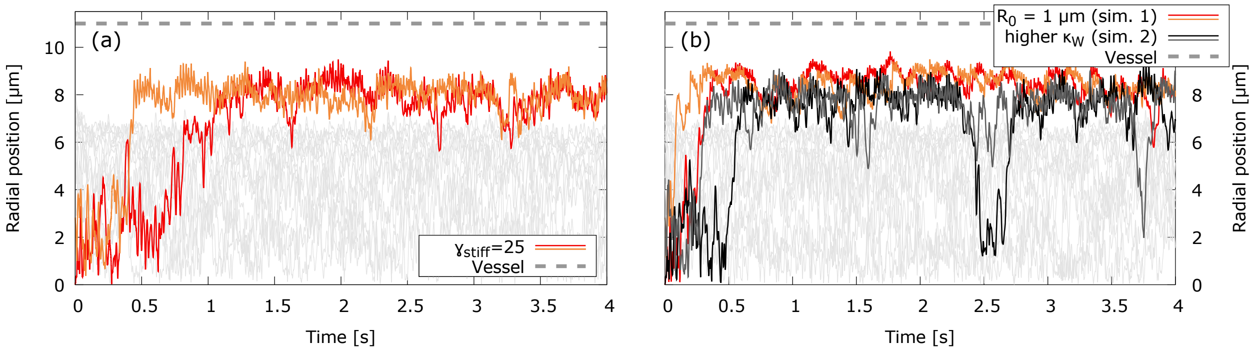


Figure S8: Behavior of two oscillating lipid coated microbubbles for $\delta = 1$, $f = 1$ kHz and $P_A = 6$ kPa with red blood cells. The primary radiation force is included ($|F_{rad}| \approx 1.5 \times 10^{-17}$ N). (a) The surface tension in the stiff state is increased to $\gamma_{stiff} = 25\kappa_S$. (b) Two simulations, once for bubbles of half the usual size ($R_0 = 1$ µm) and once for a five times stiffer vessel wall ($\kappa_{Wall} = 31.25 \times 10^6$ N/m$^3$). The qualitative results remain unchanged in all cases.

# S4 Code verification

We performed extensive testing of our code to ensure correctness of both the chosen algorithms as well as of the implementation itself. For example, we compared the results of the single- and double-layer integrals for both the infinite and the periodic Green's functions with analytically known values (similar to ref. [8]). The red blood cell model was validated by considering, amongst others, the deformation of a capsule in an infinite shear flow, as published in reference [7] and further explored below, as well as by comparing with analytical calculations for a diffusing particle near elastic membranes [9–14]. We also used the code to compute the shapes assumed by red blood cells in microchannels [15].

For further verifications we consider a single bubble in an extensional flow in figure S9. More precisely, the flow is solved with VCO-BIM in an infinite domain ($V_\Gamma \to \infty$) as explained in the main text with the imposed

flow set to $\boldsymbol{u}^{\infty}(\boldsymbol{x}) = s\,(2x, -y, -z)$, where $s$ is the shear rate (for infinite domains, more general imposed flows $\boldsymbol{u}^{\infty}(\boldsymbol{x})$ are possible instead of only a constant flow $\langle \boldsymbol{u} \rangle_{\Gamma}$ [16]). The bubble starts with 5120 triangles and is refined as needed [17]. Moreover, the mean curvature is computed via Method C from ref. [7] and the mesh stabilization routine from equation (2.72) from the main text is employed. The proper dimensionless parameter is the capillary number $\mathrm{Ca} = s\mu R/\gamma$, where $\mu$ is the dynamic viscosity of the ambient fluid, $R$ the initial bubble radius and $\gamma$ the surface tension. For comparison with the literature, we extract the Taylor deformation parameter $D = (a-c)/(a+c)$. The length of the largest half-axis $a$ and of the smallest half-axis $c$ of the deformed object are computed from an ellipsoid with the same inertia tensor [18, 19]. Figure S9 (a) shows a cut through the bubble in the $z = 0$ plane in the stationary state and compares it with the shapes found by Youngren and Acrivos using an axisymmetric boundary integral method [20]. Furthermore, figure S9 (b) depicts the stationary value for the deformation parameter $D$ as a function of the capillary number. We compare it with the numerical results of Youngren and Acrivos [20] and with the analytical $\mathcal{O}(\mathrm{Ca}^2)$ theory of Barthès-Biesel and Acrivos [21]. In both cases very good agreement is observed. We also note that the deformation in the $\mathrm{Ca} = 0.1$ case corresponds to an asphericity of around 0.295, which is larger than any values observed for the full setup from the main text. Hence we conclude that we obtain correct behavior within the relevant deformation range.

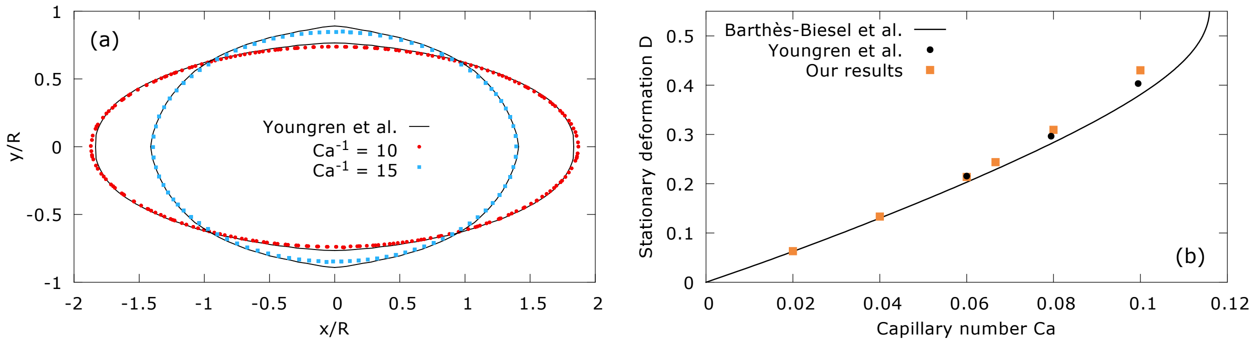


Figure S9: Verification of the bubble in an infinite extensional flow. (a) Cut through the stationary 3D shape of the bubble in the $z = 0$ plane for two different capillary numbers. The black lines depict the results obtained by Youngren and Acrivos using an axisymmetric boundary integral method [20]. (b) Stationary Taylor deformation parameter $D$ as a function of the capillary number. The black dots depict the result by Youngren and Acrivos [20], the orange squares our results. Furthermore, we show the analytical theory of Barthès-Biesel and Acrivos as a black line [21]. Note that it quickly diverges contrary to numerical evidence [20]. Hence, its validity appears to be limited to $\mathrm{Ca} \lesssim 0.06$ where excellent agreement is found.

In reference [7] we treated the case of a capsule in an infinite shear flow, and found very good matching with the literature (figures 12 and 17 therein). For the *periodic* system we show a similar result in figure S10. Namely, we place two flat walls with a distance $h = 19R$ in a cubic unit cell with side lengths $20R$ together with an initially spherical capsule of radius $R$. We implement the shear flow by prescribing the velocities $\boldsymbol{u} = (\pm sh/2, 0, 0)$ at the walls, whereas the top (bottom) sign corresponds to the top (bottom) wall and $s$ is the shear rate. The capsule is endowed not only with some shear elasticity modeled according to the neo-Hookean law (shear modulus $\kappa_{\mathrm{S}}$ [7]), but also with some bending rigidity following the Canham-Helfrich law [22–24] (bending modulus $\kappa_{\mathrm{B}}$, Method C from ref. [7], flat reference state). We set the inner viscosity to be identical to the dynamic viscosity $\mu$ of the ambient fluid. Hence, two dimensionless parameters are relevant: The capillary number $\mathrm{Ca} = s\mu R/\kappa_{\mathrm{S}}$ and the reduced bending modulus $\hat{\kappa}_{\mathrm{B}} = \kappa_{\mathrm{B}}/(R^2\kappa_{\mathrm{S}})$. As before, we extract the Taylor deformation parameter $D$. See reference [7] for further details and section 3.2 in the main text for the remaining parameters. Varying the distance between the walls does not change the results significantly compared to $h = 19R$. We therefore effectively mimic an infinite system and comparisons with results from unbounded flows are appropriate. However, the keypoint here is that we use the very same SPME code that is also employed for the simulations in the main paper, and thereby further validate the implementation. Numerical parameters include 1280 triangles for the capsule (which is well converged [7] and roughly corresponds to the maximal resolution used for the red blood cells in the margination simulations) and 800 triangles per wall. The SPME error is $\lesssim 0.01\,\%$ (similar to the main simulations). Obviously, figure S10 shows that our results compare very favorably with data extracted from Tsubota [25], proving that our code works as intended.

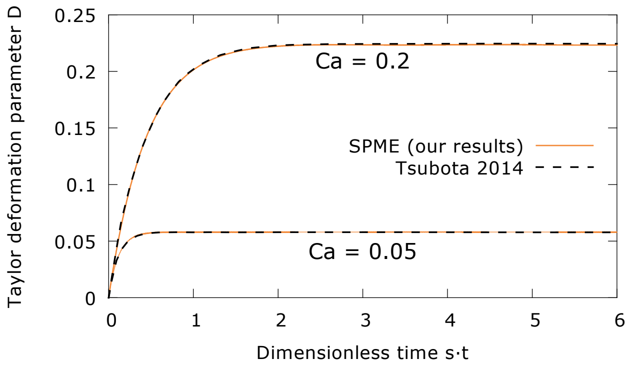


Figure S10: Deformation of a single spherical capsule (endowed with shear elasticity and bending rigidity) in a periodic system for two different capillary numbers Ca, compared to results from reference [25] ("model H" therein). We set $\hat{\kappa}_B = 2/15$. Since the wall distance $h$ is chosen sufficiently large, the data matches very well although the values from the literature were obtained for a capsule in an infinite (rather than a periodic) system.

# S5 Dynamic mesh refinement

As outlined in the main text, we employ Rivara's longest-edge bisection algorithm [17] in order to refine the triangular meshes locally when objects come close to each other and at high curvature regions. Lower resolutions are sufficient for the other regions, i.e. we coarsen the previously refined areas again in this case. Example snapshots are shown in figure S11.

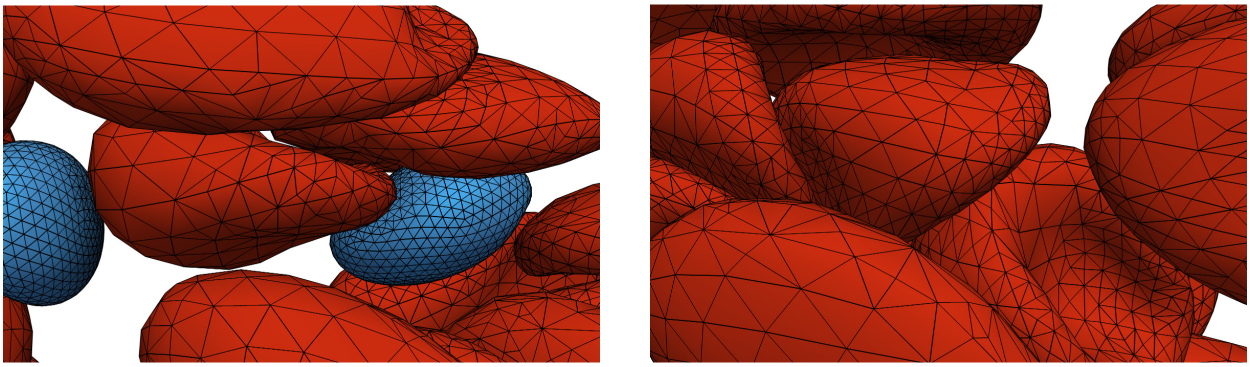

Figure S11: Example snapshots from the simulations, highlighting the dynamic mesh refinement due to close contact and high curvature regions.

# References

[1] K. Müller, D. A. Fedosov, and G. Gompper, *"Margination of micro- and nano-particles in blood flow and its effect on drug delivery,"* Sci. Rep. **4**, 4871 (2014).

[2] P. Dayton, A. Klibanov, G. Brandenburger, and K. Ferrara, *"Acoustic radiation force in vivo: A mechanism to assist targeting of microbubbles,"* Ultrasound Med. Biol. **25**, 1195 (1999).

[3] J. J. Rychak, A. L. Klibanov, K. F. Ley, and J. A. Hossack, *"Enhanced Targeting of Ultrasound Contrast Agents Using Acoustic Radiation Force,"* Ultrasound. Med. Biol. **33**, 1132 (2007).

[4] K. A. Johnson, H. R. Vormohr, A. A. Doinikov, A. Bouakaz, C. W. Shields, G. P. López, and P. A. Dayton, *"Experimental verification of theoretical equations for acoustic radiation force on compressible spherical particles in traveling waves,"* Phys. Rev. E **93**, 053109 (2016).

[5] A. Prosperetti, *"Bubble phenomena in sound fields: Part two,"* Ultrasonics **22**, 115 (1984).

[6] P. Marmottant, S. van der Meer, M. Emmer, M. Versluis, N. de Jong, S. Hilgenfeldt, and D. Lohse, *"A model for large amplitude oscillations of coated bubbles accounting for buckling and rupture,"* J. Acoust. Soc. Am. **118**, 3499 (2005).

[7] A. Guckenberger, M. P. Schraml, P. G. Chen, M. Leonetti, and S. Gekle, *"On the bending algorithms for soft objects in flows,"* Comput. Phys. Comm. **207**, 1 (2016).

[8] A. Farutin, T. Biben, and C. Misbah, *"3D numerical simulations of vesicle and inextensible capsule dynamics,"* J. Comput. Phys. **275**, 539 (2014).

[9] A. Daddi-Moussa-Ider, A. Guckenberger, and S. Gekle, *"Long-lived anomalous thermal diffusion induced by elastic cell membranes on nearby particles,"* Phys. Rev. E **93**, 012612 (2016).

[10] A. Daddi-Moussa-Ider, A. Guckenberger, and S. Gekle, *"Particle mobility between two planar elastic membranes: Brownian motion and membrane deformation,"* Phys. Fluids **28**, 071903 (2016).

[11] A. Daddi-Moussa-Ider and S. Gekle, *"Hydrodynamic interaction between particles near elastic interfaces,"* J. Chem. Phys. **145**, 014905 (2016).

[12] A. Daddi-Moussa-Ider, M. Lisicki, and S. Gekle, *"Mobility of an axisymmetric particle near an elastic interface,"* J. Fluid Mech. **811**, 210 (2017).

[13] A. Daddi-Moussa-Ider and S. Gekle, *"Hydrodynamic mobility of a solid particle near a spherical elastic membrane: Axisymmetric motion,"* Phys. Rev. E **95**, 013108 (2017).

[14] A. Daddi-Moussa-Ider, M. Lisicki, and S. Gekle, *"Hydrodynamic mobility of a solid particle near a spherical elastic membrane. II. Asymmetric motion,"* Phys. Rev. E **95**, 053117 (2017).

[15] S. Quint, A. F. Christ, A. Guckenberger, S. Himbert, L. Kaestner, S. Gekle, and C. Wagner, *"3D tomography of cells in micro-channels,"* Appl. Phys. Lett. **(accepted)** (2017).

[16] C. Pozrikidis, *"Interfacial Dynamics for Stokes Flow,"* J. Comput. Phys. **169**, 250 (2001).

[17] M. C. Rivara, *"Algorithms for refining triangular grids suitable for adaptive and multigrid techniques,"* Int. J. Numer. Methods Eng. **20**, 745 (1984).

[18] T. Krüger, F. Varnik, and D. Raabe, *"Efficient and accurate simulations of deformable particles immersed in a fluid using a combined immersed boundary lattice Boltzmann finite element method,"* Comput. Math. Appl. **61**, 3485 (2011).

[19] S. Ramanujan and C. Pozrikidis, *"Deformation of liquid capsules enclosed by elastic membranes in simple shear flow: Large deformations and the effect of fluid viscosities,"* J. Fluid Mech. **361**, 117 (1998).

[20] G. K. Youngren and A. Acrivos, *"On the shape of a gas bubble in a viscous extensional flow,"* J. Fluid Mech. **76**, 433 (1976).

[21] D. Barthès-Biesel and A. Acrivos, *"Deformation and burst of a liquid droplet freely suspended in a linear shear field,"* J. Fluid Mech. **61**, 1 (1973).

[22] P. B. Canham, *"The minimum energy of bending as a possible explanation of the biconcave shape of the human red blood cell,"* J. Theor. Biol. **26**, 61 (1970).

[23] W. Helfrich, *"Elastic Properties of Lipid Bilayers: Theory and Possible Experiments,"* Z. Naturforsch. C **28**, 693 (1973).

[24] A. Guckenberger and S. Gekle, *"Theory and algorithms to compute Helfrich bending forces: A review,"* J. Phys. Condens. Matter **29**, 203001 (2017).

[25] K.-i. Tsubota, *"Short note on the bending models for a membrane in capsule mechanics: Comparison between continuum and discrete models,"* J. Comput. Phys. **277**, 320 (2014).
